# Supplementary material for: Qualitative Insight and Quantitative Analysis of the Effect of Temperature on the Coercivity of a Magnetic System
Source: arXiv:1512.01962 source file (2015-12-07)
Supplement: Supplementary file 1 [file suppl.pdf]

# Qualitative Insight and Quantitative Analysis of the Effect of Temperature on the Coercivity of a Magnetic System

Mariia Moskalenko,[1,2] Pavel F. Bessarab,[3,4,*] Valery M. Uzdin,[2,4] and Hannes Jónsson[1,5]

[1]*Science Institute and Faculty of Physical Sciences, Univ. of Iceland, 107 Reykjavík, Iceland*

[2]*St. Petersburg National Research University of Information Technologies, Mechanics and Optics, St. Petersburg, 197101, Russia*

[3]*Dept. of Materials and Nanophysics, Electrum 229, Royal Institute of Technology (KTH), SE-16440 Kista, Sweden*

[4]*Department of Physics, St. Petersburg State University, St. Petersburg, 198504, Russia*

[5]*Department of Applied Physics, Aalto University, Espoo, FIN-00076, Finland*

[*] E-mail: bessarab@kth.se; Corresponding author

## S1. LIFETIME OF A MAGNETIC STATE

The harmonic approximation to transition state theory (HTST) is used to calculate the lifetime of a magnetic state [1]:

$$\tau^{HTST} = \nu^{-1} e^{(\mathcal{E}_s - \mathcal{E}_m)/k_B T}. \tag{S1}$$

Here, $\mathcal{E}_m$ and $\mathcal{E}_s$ is the energy of the initial state and the saddle point (SP) configuration, respectively. The pre-exponential factor, $\nu$, is calculated based on the assumption that magnetization dynamics in the vicinity of the SP is described by linearized Landau-Lifshitz equations of motion.

For a spring magnet divided into $N$ layers, where magnetization within each layer does not change upon rotation of the moments and both minimum energy and SP configurations correspond to an in-plane alignment of the moments (so that all polar angles $\theta_i$ defining orientation of magnetization within each atomic layer of the spring magnet can be set to $\pi/2$), the pre-exponential factor is given by [1]:

$$\nu = \frac{\gamma}{2\pi} \sqrt{\sum_{i=2}^{2N} \frac{a_i^2}{\epsilon_i}} \sqrt{\frac{\det H_m}{\det' H_s}} \tag{S2}$$

where $\gamma$ is the gyromagnetic ratio, $\det H_m$ and $\det H_s$ denote the determinants of the Hessian matrices at the spiral state minimum and at the SP, respectively, $\epsilon_i$ are the eigenvalues of the Hessian at the SP, and $a_i$ are expansion coefficients in the linearized equation for the unstable mode derived from the set of equations of motion for $2N$ dynamical variables of the spring magnet [1]. Spherical coordinates, $\theta_i$ and $\phi_i$, defining the orientation of the magnetization within each layer $i$ have been chosen as dynamical variables. The determinants in Eq. (S2) are computed as a product of the eigenvalues and the prime means that the negative one, $\epsilon_1$, is omitted. $H_m$ and $H_s$ are $2N \times 2N$ matrices of second derivatives of the energy with respect to spherical coordinates computed at the minimum and at the SP, respectively.

Direct application of the Geodesic Nudged Elastic Band (GNEB) method [2] to one-dimensional, multilayer model of a spring magnet (see Eq. (1) in the main body of the Article) gives activation energy per unit area, $E_a = E_s - E_m$, where indices $m$ and $s$ denote the spiral state and the saddle point (SP) configuration, respectively. In order to estimate an absolute value of the activation energy, $\mathcal{E}_a = S_\perp E_a$, the relevant area, $S_\perp$, where the

nucleation of the collinear state takes place needs to be estimated. This analysis is given in the Supplemental Section S3.

The multilayer model of the spring magnet assumes in-plane rotation of the magnetization within each layer, so that only $N$ configuration parameters, the azimuthal angles $\phi_i$, are included, while the polar angles $\theta_i$ are kept fixed at $\theta_i = \pi/2$ for all the layers. This is sufficient for finding activation energy, $\mathcal{E}_a$, provided that the nucleation area, $S_\perp$, is known. Supplemental Eq. (S2) for the pre-exponential factor requires, however, an extension of the model so as to include the whole set of $2N$ configuration parameters. This extension is presented in Supplemental Section S2. Supplemental Eq. (S2) further shows that $\nu$ is independent of the nucleation area, so $S_\perp$ is not needed for the calculation of the pre-exponential factor.

## S2. EVALUATION OF THE PRE-EXPONENTIAL FACTOR

The $2N \times 2N$ Hessian matrices $H_m$ and $H_s$ as well as expansion coefficients $a_i$ in Supplemental Eq. (S2) are only well defined when the whole set of $2N$ configuration parameters, the spherical coordinates $(\theta_1, \phi_1, \ldots, \theta_N, \phi_N)$, are included in the model of the system. Therefore, the model of a spring magnet described by Eq. (1) of the main body of the Article needs to be extended by adding easy plane anisotropy and including the $\theta_i$ variables in the energy expression. The extended Hamiltonian is:

$$E = -\sum_{i=1}^{N-1} \frac{A_\alpha}{d} \left[\sin(\theta_i)\sin(\theta_{i+1})\cos(\phi_i - \phi_{i+1}) + \cos(\theta_i)\cos(\theta_{i+1})\right] \\ - d\sum_{i=1}^{N} K_\beta \sin^2(\theta_i)\cos^2(\phi_i) - d\sum_{i=1}^{N} HM_\beta \sin(\theta_i)\cos(\phi_i - \phi_H) + 2\pi d \sum_{i=1}^{N} M_\beta^2 \cos^2(\theta_i). \tag{S3}$$

Here, $M_\beta$ and $K_\beta$ are the magnetization and anisotropy constant, respectively, in the soft ($\beta = s$) and hard ($\beta = h$) magnet, $d$ is the distance between atomic layers, $A_\alpha$ is the exchange coupling between adjacent layers in the soft magnet ($\alpha = s$), hard magnet ($\alpha = h$) and at the interface ($\alpha = int$), $\phi_H$ is the angle the external field $H$ make with the anisotropy axis and $N$ is the total number of atomic layers. Supplemental Eq. (S3) reduces to Eq. (1) when all $\theta_i$ are set to $\pi/2$. The last term in Supplemental Eq. (S3) represents the shape anisotropy of a thin film [3] which makes it preferable for the magnetization to lie in the plane

of the film. This last term ensures that minima and SPs of the energy surface described by Supplemental Eq. (S3) coincide with those given by the reduced model defined by Eq. (1). Numerical values of the parameters in Supplemental Eq. (S3) are taken from ref. [4], except for a 20% increase in $K_h$, as described in the Article: $A_h = 1.2 \times 10^{-6}$ ergs/cm, $K_h = 6 \times 10^7$ ergs/cm$^3$, $M_h = 550$ emu/cm$^3$, $A_s = 2.8 \times 10^{-6}$ ergs/cm, $K_s = 10^3$ ergs/cm$^3$, $M_s = 1700$ emu/cm$^3$, $A_{int} = 1.8 \times 10^{-6}$ ergs/cm, $\phi_H = 3°$, $d = 2$ Å, $N = N_s + N_h = 240$. The number of atomic layers in the soft magnet, $N_s$, was taken to be 100, while the number of atomic layers in the hard magnet, $N_h$, was set to 140.

The pre-exponential factor $\nu$ is calculated in the following way. The spiral state minimum, $(\phi_1^m, \ldots, \phi_N^m)$, and the SP configuration, $(\phi_1^s, \ldots, \phi_N^s)$, are identified for the reduced model given by Eq. (3). These configurations are used to define the energy minimum and the SP states in the extended model, where polar angles defining orientation of magnetization in each layer are set to $\pi/2$. Finally, Supplemental Eq. (S3) is used to compute the Hessian matrices $H_m$ and $H_s$ and the expansion coefficients $a_i$ in Supplemental Eq. (S2). The calculated pre-exponential factor is shown in Supplemental Fig. 1 as a function of the external field. We note that the value of the prefactor is only weakly dependent on the choice of the plane anisotropy. An order of magnitude change in the anisotropy constant only changes the prefactor by a factor of two.

## S3. ESTIMATION OF THE NUCLEATION AREA

The nucleation area, $S_\perp$, can be estimated based on the experimental value of the coercivity, $H_{irr}$, at a given temperature, as described below. Given a time scale of the experiment, $\tau_{exp}$, the coercivity at temperature $T$ is implicitly given by

$$\tau(T, H_{irr}) = \tau_{exp}. \tag{S4}$$

The coercivity is the magnitude of the external field at which the time scale of thermally activated transitions from the spiral state to the homogeneous state, $\tau(T, H_{irr})$, becomes equal to the time scale of the experiment. This is analogous to Eqn. (12) of Suess et al. in Ref. [5]. Within HTST, both the activation energy and the pre-exponential factor are field dependent:

$$\tau(T, H) = \nu^{-1}(H) \exp\left[E_a(H) S_\perp / k_B T\right]. \tag{S5}$$

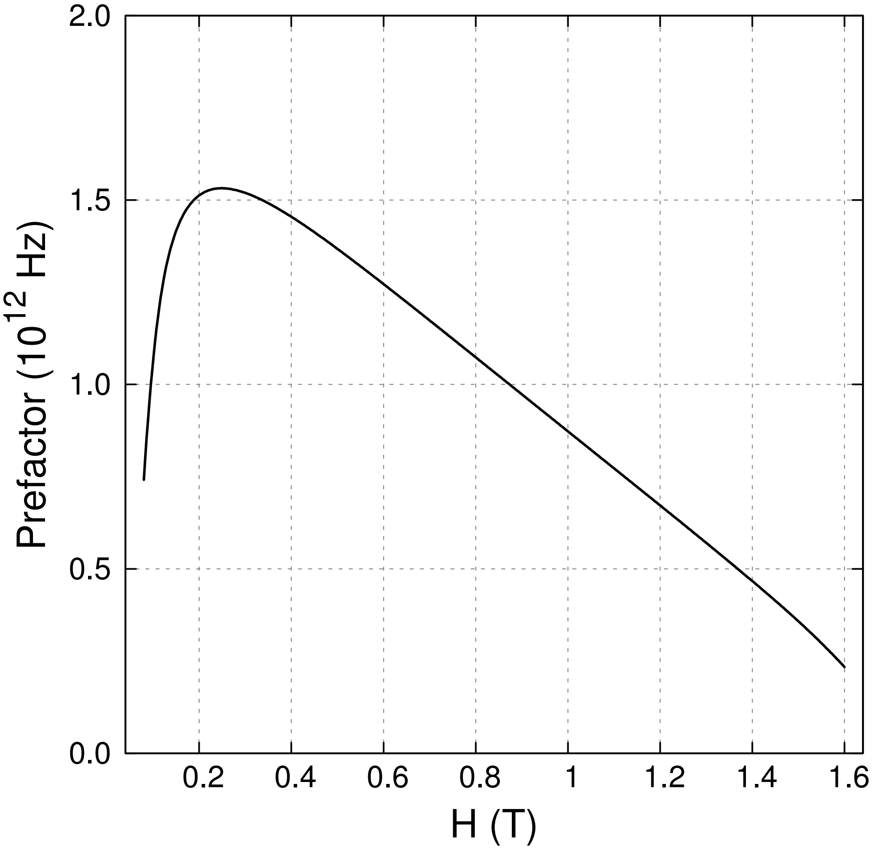


Supplemental Figure 1. Pre-exponential factor, $\nu$, as a function of the external magnetic field.

From Supplemental Eqs. (S4)-(S5) it follows that

$$S_{\perp} = \frac{k_B T \ln\left[\nu(H_{irr})\tau_{exp}\right]}{E_a(H_{irr})}. \tag{S6}$$

$E_a(H_{irr})$ is found directly from the GNEB calculations, while $\nu(H_{irr})$ is calculated using Supplemental Eq. (S2) (see also Supplemental Section S2). Using experimental value of $H_{irr} = 1.45$ T at $T = 25$ K and assuming $\tau_{exp} = 1$ s, the nucleation area $S_{\perp}$ is found to be 20 nm$^2$. This value can then be used to predict the $H_{irr}$ at any temperature. A graphical solution of Supplemental Eq. (S4) with the lifetime given by Supplemental Eq. (S5) is shown in Supplemental Fig. 2.

[1] P.F. Bessarab, V.M. Uzdin and H. Jónsson, Harmonic Transition State Theory of Thermal Spin Transitions. Phys. Rev. B **85**, 184409 (2012).

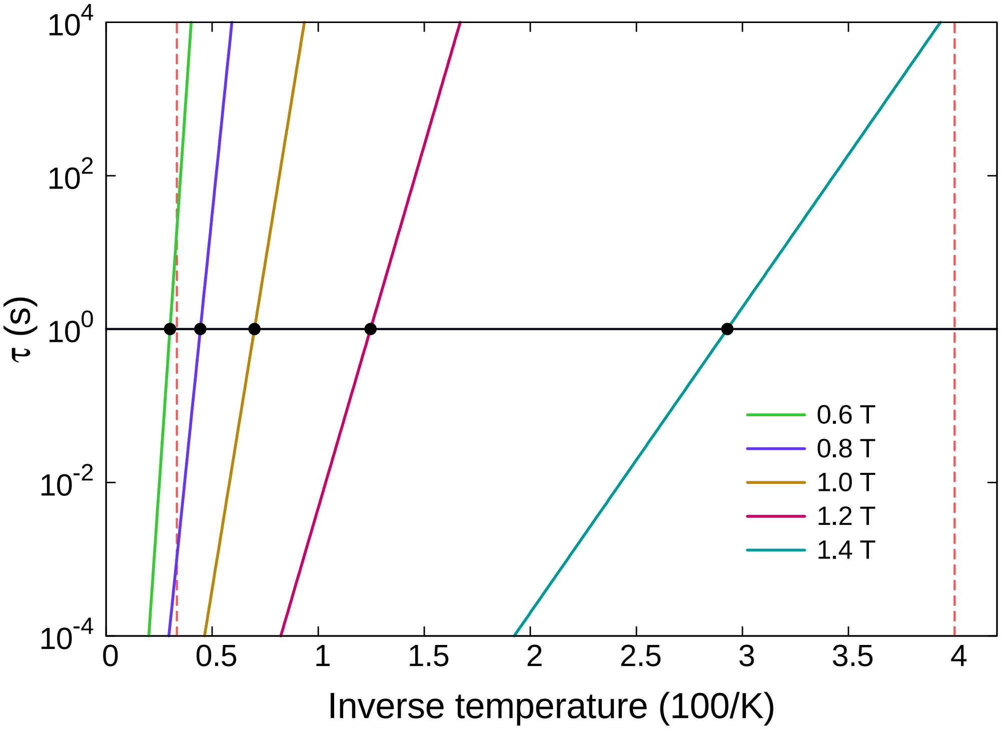


Supplemental Figure 2. Time scale of thermally activated escape from the spiral state as a function of inverse temperature for five values of the external field, ranging from 0.6 T to 1.4 T. The intersections with the level $\tau = 1$ s (marked with filled circles) define the temperature at which the given field strength lowers the activation energy sufficiently to make the thermal transition occur on the time scale of 1 s. Vertical dashed lines correspond to 25 K and 300 K.

[2] P.F. Bessarab, V.M. Uzdin and H. Jónsson, Method for finding mechanism and activation energy of magnetic transitions, applied to skyrmion and antivortex annihilation. *Comput. Phys. Commun.* in press, 2015. (Manuscript available at http://arxiv.org/abs/1502.05065).

[3] M.T. Johnson, P.J.H. Bloemen, F.J.A. den Broeder, and J.J. de Vries, Magnetic anisotropy in metallic multilayers. Rep. Prog. Phys. **59**, 1409 (1996).

[4] E.E. Fullerton, J.S. Jiang, M. Grimsditch, C.H. Sowers and S.D. Bader, Exchange-spring behavior in epitaxial hard/soft magnetic bilayers. Phys. Rev. B **58**, 12193 (1998).

[5] D. Suess, L. Breth, J. Lee, M. Fuger, C. Vogler, F. Bruckner, B. Bergmair, T. Huber, J. Fidler and T. Schrefl, Calculation of Coercivity of Magnetic Nanostructures at Finite Temperatures. *Phys. Rev. B* **84** 224421 (2011).
